# Supplementary material for: Parallel $k$d-tree with Batch Updates
Source: arXiv:2411.09275 source file (2025-01-06)
Supplement: Supplementary file 3 [file appendix-perf-hardware-table-full.tex]

\begin{table}[t]
	\centering
	% \Huge
	% \resizebox{.48\textwidth}{!}{

	\small
	\setlength\tabcolsep{1.6pt}

	% Table generated by Excel2LaTeX from sheet 'revis-perf'
	\begin{tabular}{cc|ccccccc}
		\toprule
		                                                       & \textbf{Baselines} & \textbf{CC(M)}      & \textbf{Inst(M)}   & \textbf{IPC}     & \textbf{CRs(M)} & \textbf{CMs(M)} & \textbf{BR(M)}    & \textbf{BMs(M)}  \\
		\midrule
		\multirow{5}[2]{*}{\begin{sideways}HT\end{sideways}}   & \ours{}               & 95,300              & 31,084             & .326             & 926             & 508             & 6,832             & 58.0             \\
		                                                       & \oursbb{}            & \underline{33,885}  & \underline{17,143} & .506             & \underline{245} & 134             & \underline{2,279} & \underline{17.9} \\
		                                                       & \bhltree{}         & 41,969              & 31,091             & \underline{.741} & 254             & \underline{132} & 3,254             & 18.3             \\
		                                                       & \logtree{}         & 40,937              & 26,280             & .642             & 362             & 179             & 2,825             & 23.0             \\
		                                                       & \cgal{}            & 3,647,256           & 46,255             & .013             & 1,506           & 824             & 11,098            & 171              \\
		\midrule
		\multirow{5}[2]{*}{\begin{sideways}HH\end{sideways}}   & \ours{}               & 69,078              & 22,127             & .320             & 557             & 361             & 4,114             & 117              \\
		                                                       & \oursbb{}            & \underline{27,987}  & \underline{10,831} & .387             & \underline{242} & \underline{150} & \underline{1,636} & \underline{43.9} \\
		                                                       & \bhltree{}         & 38,846              & 39,413             & \underline{1.01} & 424             & 189             & 4,670             & 75.2             \\
		                                                       & \logtree{}         & 43,343              & 34,957             & .807             & 649             & 285             & 4,510             & 120              \\
		                                                       & \cgal{}            & n.a.                & n.a.               & n.a.             & n.a.            & n.a.            & n.a.              & n.a.             \\
		\midrule
		\multirow{5}[2]{*}{\begin{sideways}CHEM\end{sideways}} & \ours{}               & 243,014             & 65,919             & .271             & 1,662           & 1,450           & 14,318            & 170              \\
		                                                       & \oursbb{}            & \underline{139,701} & \underline{32,887} & .235             & \underline{954} & \underline{820} & \underline{6,583} & 107              \\
		                                                       & \bhltree{}         & 145,127             & 101,292            & \underline{.698} & 1,336           & 938             & 11,558            & 93.3             \\
		                                                       & \logtree{}         & 244,588             & 145,273            & .594             & 1,990           & 1,370           & 15,734            & 94.9             \\
		                                                       & \cgal{}            & 5,888,513           & 100,528            & .017             & 3,105           & 2,110           & 24,545            & \underline{38.8} \\
		\midrule
		\multirow{5}[2]{*}{\begin{sideways}GL\end{sideways}} & \ours{}               & 71,844              & 21,767             & .303             & 439             & 345             & 3,376             & 118              \\
		                                                       & \oursbb{}            & \underline{62,637}  & \underline{13,438} & .215             & \underline{407} & \underline{317} & \underline{1,981} & 101              \\
		                                                       & \bhltree{}         & 83,324              & 68,574             & \underline{.823} & 563             & 364             & 7,386             & \underline{45.1} \\
		                                                       & \logtree{}         & 96,609              & 65,256             & .676             & 868             & 548             & 7,329             & 76.4             \\
		                                                       & \cgal{}            & n.a.                & n.a.               & n.a.             & n.a.            & n.a.            & n.a.              & n.a.             \\
		\midrule
		\multirow{5}[2]{*}{\begin{sideways}CM\end{sideways}}   & \ours{}               & \underline{120,478} & 22,407             & .186             & \underline{692} & \underline{649} & 3,397             & 173              \\
		                                                       & \oursbb{}            & 133,104             & \underline{21,913} & .165             & 752             & 703             & \underline{3,296} & 176              \\
		                                                       & \bhltree{}         & 134,563             & 79,771             & .593             & 1,359           & 1,139           & 9,635             & \underline{158}  \\
		                                                       & \logtree{}         & 160,625             & 95,983             & \underline{.598} & 2,035           & 1,614           & 11,766            & 210              \\
		                                                       & \cgal{}            & 33,290,752          & 110,315            & .003             & 7,290           & 4,040           & 26,484            & 979              \\
		\midrule
		\multirow{5}[2]{*}{\begin{sideways}OSM\end{sideways}}  & \ours{}               & \underline{71,679}  & 12,247             & .171             & \underline{460} & \underline{426} & 1,366             & 49.7             \\
		                                                       & \oursbb{}            & 75,185              & \underline{11,124} & .148             & 473             & 441             & \underline{1,178} & \underline{47.8} \\
		                                                       & \bhltree{}         & 127,065             & 72,183             & .568             & 1,710           & 1,294           & 10,448            & 53.2             \\
		                                                       & \logtree{}         & 190,718             & 121,444            & \underline{.637} & 2,687           & 1,882           & 16,399            & 79.7             \\
		                                                       & \cgal{}            & 47,746,792          & 111,702            & .002             & 9,287           & 5,168           & 27,005            & 895              \\
		\bottomrule
	\end{tabular}%

	% }
	\caption{
		\textbf{Hardware profiling of benchmarks for range report query on real-world datasets.
			Unerlined values indicate better performance.
		}
		The range report query contains $10^4$ rectangles each with output size $10^4$--$10^6$. Different queries are performed in parallel, and each query searches the tree in serial.
		``\oursbb{}'': The \ourlib{} with bounding box stored in every node.
		``CC'': Cycles, ``Inst'': Instructions, ``IPC'': Instructions per cycle, ``CR'': Cache reference, ``CMs'': Cache misses, ``BR'': Branches, ``BMs'': Branch misses.
		%\ziyang{this table now becomes table 1. The first table in main paper is table 2.}
	}

	\label{table:appendix:perf-hardware-full}%
\end{table}%
